# Supplementary material for: Action Motifs: Self-Supervised Hierarchical Representation of Human Body Movements
Source: arXiv:2604.28173 source file (2026-06-02)
Supplement: Supplementary file 1 [file suppl_amd_samples.tex]

\begin{tikzpicture}[x=1mm,y=1mm,every node/.style={inner sep=0pt, text depth=0pt}]
    \newcount\colwidth \colwidth=35  % 各列の幅
    \newcount\rowheight \rowheight=-27 % 各行の高さ

    \newcount\vx \vx=0
    \newcount\vy \vy=0

    \newcommand\imagewidth{0.20\textwidth} % 主画像の幅

    \def\Pa#1{\includegraphics[width=\imagewidth,bb={126 81 574 417},clip]{#1}}
    \def\Pb#1{\includegraphics[width=\imagewidth,bb={206 261 736 659},clip]{#1}}
    \def\Pc#1{\includegraphics[width=\imagewidth,bb={46 281 494 617},clip]{#1}}
    \def\Pd#1{\includegraphics[width=\imagewidth,bb={66 41 862 637},clip]{#1}}
    \def\Pe#1{\includegraphics[width=\imagewidth,bb={246 312 694 648},clip]{#1}}
    \def\Pf#1{\includegraphics[width=\imagewidth,bb={273 207 864 648},clip]{#1}}
    \def\Pg#1{\includegraphics[width=\imagewidth,bb={308 232 864 648},clip]{#1}}
    \def\Ph#1{\includegraphics[width=\imagewidth,bb={0 0 864 648},clip]{#1}}

    % % --- 1行目の画像 ---
    \vy = 0
    \node[anchor=north] at (\vx, \vy) {\Pa{fig/smpl_lemo_without_penetration_final_final_final_final_rendering_supp/2024-09/17/batch1/b-3/gopro11/3/0000001601.jpg}}; \advance \vx by \colwidth
    \node[anchor=north] at (\vx, \vy) {\Pa{fig/smpl_lemo_without_penetration_final_final_final_final_rendering_supp/2024-09/17/batch1/b-3/gopro11/3/0000001611.jpg}}; \advance \vx by \colwidth
    \node[anchor=north] at (\vx, \vy) {\Pa{fig/smpl_lemo_without_penetration_final_final_final_final_rendering_supp/2024-09/17/batch1/b-3/gopro11/3/0000001621.jpg}}; \advance \vx by \colwidth
    \node[anchor=north] at (\vx, \vy) {\Pa{fig/smpl_lemo_without_penetration_final_final_final_final_rendering_supp/2024-09/17/batch1/b-3/gopro11/3/0000001631.jpg}}; \advance \vx by \colwidth
    \node[anchor=north] at (\vx, \vy) {\Pa{fig/smpl_lemo_without_penetration_final_final_final_final_rendering_supp/2024-09/17/batch1/b-3/gopro11/3/0000001641.jpg}}; \advance \vx by \colwidth

    \vx = 0
    \advance \vy by \rowheight
    \node[anchor=north] at (\vx, \vy) {\Pb{fig/smpl_lemo_without_penetration_final_final_final_final_rendering_supp/2024-09/19/batch2/a-1/gopro11/3/0000002467.jpg}}; \advance \vx by \colwidth
    \node[anchor=north] at (\vx, \vy) {\Pb{fig/smpl_lemo_without_penetration_final_final_final_final_rendering_supp/2024-09/19/batch2/a-1/gopro11/3/0000002477.jpg}}; \advance \vx by \colwidth
    \node[anchor=north] at (\vx, \vy) {\Pb{fig/smpl_lemo_without_penetration_final_final_final_final_rendering_supp/2024-09/19/batch2/a-1/gopro11/3/0000002487.jpg}}; \advance \vx by \colwidth
    \node[anchor=north] at (\vx, \vy) {\Pb{fig/smpl_lemo_without_penetration_final_final_final_final_rendering_supp/2024-09/19/batch2/a-1/gopro11/3/0000002497.jpg}}; \advance \vx by \colwidth
    \node[anchor=north] at (\vx, \vy) {\Pb{fig/smpl_lemo_without_penetration_final_final_final_final_rendering_supp/2024-09/19/batch2/a-1/gopro11/3/0000002507.jpg}}; \advance \vx by \colwidth

    \vx = 0
    \advance \vy by \rowheight
    \node[anchor=north] at (\vx, \vy) {\Pc{fig/smpl_lemo_without_penetration_final_final_final_final_rendering_supp/2024-09/19/batch2/a-3/gopro11/1/0000000316.jpg}}; \advance \vx by \colwidth
    \node[anchor=north] at (\vx, \vy) {\Pc{fig/smpl_lemo_without_penetration_final_final_final_final_rendering_supp/2024-09/19/batch2/a-3/gopro11/1/0000000326.jpg}}; \advance \vx by \colwidth
    \node[anchor=north] at (\vx, \vy) {\Pc{fig/smpl_lemo_without_penetration_final_final_final_final_rendering_supp/2024-09/19/batch2/a-3/gopro11/1/0000000336.jpg}}; \advance \vx by \colwidth
    \node[anchor=north] at (\vx, \vy) {\Pc{fig/smpl_lemo_without_penetration_final_final_final_final_rendering_supp/2024-09/19/batch2/a-3/gopro11/1/0000000346.jpg}}; \advance \vx by \colwidth
    \node[anchor=north] at (\vx, \vy) {\Pc{fig/smpl_lemo_without_penetration_final_final_final_final_rendering_supp/2024-09/19/batch2/a-3/gopro11/1/0000000356.jpg}}; \advance \vx by \colwidth

    \vx = 0
    \advance \vy by \rowheight
    \node[anchor=north] at (\vx, \vy) {\Pd{fig/smpl_lemo_without_penetration_final_final_final_final_rendering_supp/2024-10/10/batch1/a-2/gopro11/6/0000004337.jpg}}; \advance \vx by \colwidth
    \node[anchor=north] at (\vx, \vy) {\Pd{fig/smpl_lemo_without_penetration_final_final_final_final_rendering_supp/2024-10/10/batch1/a-2/gopro11/6/0000004342.jpg}}; \advance \vx by \colwidth
    \node[anchor=north] at (\vx, \vy) {\Pd{fig/smpl_lemo_without_penetration_final_final_final_final_rendering_supp/2024-10/10/batch1/a-2/gopro11/6/0000004347.jpg}}; \advance \vx by \colwidth
    \node[anchor=north] at (\vx, \vy) {\Pd{fig/smpl_lemo_without_penetration_final_final_final_final_rendering_supp/2024-10/10/batch1/a-2/gopro11/6/0000004352.jpg}}; \advance \vx by \colwidth
    \node[anchor=north] at (\vx, \vy) {\Pd{fig/smpl_lemo_without_penetration_final_final_final_final_rendering_supp/2024-10/10/batch1/a-2/gopro11/6/0000004357.jpg}}; \advance \vx by \colwidth

    \vx = 0
    \advance \vy by \rowheight
    \node[anchor=north] at (\vx, \vy) {\Pe{fig/smpl_lemo_without_penetration_final_final_final_final_rendering_supp/2024-10/10/batch2/a-2/gopro11/11/0000002855.jpg}}; \advance \vx by \colwidth
    \node[anchor=north] at (\vx, \vy) {\Pe{fig/smpl_lemo_without_penetration_final_final_final_final_rendering_supp/2024-10/10/batch2/a-2/gopro11/11/0000002865.jpg}}; \advance \vx by \colwidth
    \node[anchor=north] at (\vx, \vy) {\Pe{fig/smpl_lemo_without_penetration_final_final_final_final_rendering_supp/2024-10/10/batch2/a-2/gopro11/11/0000002875.jpg}}; \advance \vx by \colwidth
    \node[anchor=north] at (\vx, \vy) {\Pe{fig/smpl_lemo_without_penetration_final_final_final_final_rendering_supp/2024-10/10/batch2/a-2/gopro11/11/0000002885.jpg}}; \advance \vx by \colwidth
    \node[anchor=north] at (\vx, \vy) {\Pe{fig/smpl_lemo_without_penetration_final_final_final_final_rendering_supp/2024-10/10/batch2/a-2/gopro11/11/0000002895.jpg}}; \advance \vx by \colwidth

    \vx = 0
    \advance \vy by \rowheight
    \node[anchor=north] at (\vx, \vy) {\Pf{fig/smpl_lemo_without_penetration_final_final_final_final_rendering_supp/2024-10/10/batch2/b-3/gopro11/11/0000000554.jpg}}; \advance \vx by \colwidth
    \node[anchor=north] at (\vx, \vy) {\Pf{fig/smpl_lemo_without_penetration_final_final_final_final_rendering_supp/2024-10/10/batch2/b-3/gopro11/11/0000000559.jpg}}; \advance \vx by \colwidth
    \node[anchor=north] at (\vx, \vy) {\Pf{fig/smpl_lemo_without_penetration_final_final_final_final_rendering_supp/2024-10/10/batch2/b-3/gopro11/11/0000000564.jpg}}; \advance \vx by \colwidth
    \node[anchor=north] at (\vx, \vy) {\Pf{fig/smpl_lemo_without_penetration_final_final_final_final_rendering_supp/2024-10/10/batch2/b-3/gopro11/11/0000000569.jpg}}; \advance \vx by \colwidth
    \node[anchor=north] at (\vx, \vy) {\Pf{fig/smpl_lemo_without_penetration_final_final_final_final_rendering_supp/2024-10/10/batch2/b-3/gopro11/11/0000000574.jpg}}; \advance \vx by \colwidth

    \vx = 0
    \advance \vy by \rowheight
    \node[anchor=north] at (\vx, \vy) {\Pg{fig/smpl_lemo_without_penetration_final_final_final_final_rendering_supp/2024-10/10/batch3/a-1/gopro11/1/0000001947.jpg}}; \advance \vx by \colwidth
    \node[anchor=north] at (\vx, \vy) {\Pg{fig/smpl_lemo_without_penetration_final_final_final_final_rendering_supp/2024-10/10/batch3/a-1/gopro11/1/0000001972.jpg}}; \advance \vx by \colwidth
    \node[anchor=north] at (\vx, \vy) {\Pg{fig/smpl_lemo_without_penetration_final_final_final_final_rendering_supp/2024-10/10/batch3/a-1/gopro11/1/0000001997.jpg}}; \advance \vx by \colwidth
    \node[anchor=north] at (\vx, \vy) {\Pg{fig/smpl_lemo_without_penetration_final_final_final_final_rendering_supp/2024-10/10/batch3/a-1/gopro11/1/0000002022.jpg}}; \advance \vx by \colwidth
    \node[anchor=north] at (\vx, \vy) {\Pg{fig/smpl_lemo_without_penetration_final_final_final_final_rendering_supp/2024-10/10/batch3/a-1/gopro11/1/0000002047.jpg}}; \advance \vx by \colwidth

    \vx = 0
    \advance \vy by \rowheight
    \node[anchor=north] at (\vx, \vy) {\Ph{fig/smpl_lemo_without_penetration_final_final_final_final_rendering_supp/2024-10/10/batch1/a-1/gopro11/1/0000002337.jpg}}; \advance \vx by \colwidth
    \node[anchor=north] at (\vx, \vy) {\Ph{fig/smpl_lemo_without_penetration_final_final_final_final_rendering_supp/2024-10/10/batch1/a-1/gopro11/1/0000002357.jpg}}; \advance \vx by \colwidth
    \node[anchor=north] at (\vx, \vy) {\Ph{fig/smpl_lemo_without_penetration_final_final_final_final_rendering_supp/2024-10/10/batch1/a-1/gopro11/1/0000002377.jpg}}; \advance \vx by \colwidth
    \node[anchor=north] at (\vx, \vy) {\Ph{fig/smpl_lemo_without_penetration_final_final_final_final_rendering_supp/2024-10/10/batch1/a-1/gopro11/1/0000002397.jpg}}; \advance \vx by \colwidth
    \node[anchor=north] at (\vx, \vy) {\Ph{fig/smpl_lemo_without_penetration_final_final_final_final_rendering_supp/2024-10/10/batch1/a-1/gopro11/1/0000002417.jpg}}; \advance \vx by \colwidth

\end{tikzpicture}
